# Supplementary material for: Critical spin fluctuations across the superconducting dome in La$_{2-x}$Sr$_{x}$CuO$_4$
Source: arXiv:2503.13600 source file (2025-11-26)
Supplement: Supplementary file 1 [file LET_Quantum_Critical_sm_v2.pdf]

# Supplementary Materials for Critical spin fluctuations across the superconducting dome in $La_{2-x}Sr_xCuO_4$


Jacopo Radaelli,[1] Oliver J. Lipscombe,[1] Mengze Zhu,[1] J. Ross Stewart,[2] Aavishkar A. Patel,[3] Subir Sachdev,[4] and Stephen M. Hayden[1]

[1] *H.H. Wills Physics Laboratory, University of Bristol, Tyndall Avenue, Bristol BS8 1TL, United Kingdom*

[2] *ISIS Pulsed Neutron and Muon Source, Rutherford Appleton Laboratory, Didcot OX11 0QX, United Kingdom*

[3] *Center for Computational Quantum Physics, Flatiron Institute, 162 5th Avenue, New York, NY 10010, USA*

[4] *Department of Physics, Harvard University, Cambridge, MA 02138, USA*


## THEORY

### Dynamic critical scaling

The dynamic susceptibility of systems below their upper critical dimension is expected to obey the following scaling behavior:

$$\chi(q,\omega,T,t) = b^{\gamma/\nu}\chi(bq, b^z\omega, b^zT, b^{1/\nu}t), \tag{S1}$$

where $b$ is an arbitrary scaling parameter, $t$ is a tuning control parameter [$t = 0$ corresponds to the quantum critical point (QCP)], $q$ is momentum relative to ordering wavevector, $\gamma$ and $\nu$ are the usual susceptibility and correlation function exponents. That is $\chi \propto t^{-\gamma}$ and $\xi \propto t^{-\nu}$. We expect the usual scaling relationship $\gamma = (2-\eta)\nu$.

*Dynamic scaling at the ordering wavevector and QCP.* We suppose to be at the QCP ($t = 0$) and consider the ordering wavevector ($q = 0$). For the imaginary part of susceptibility we have

$$\chi''(q=0,\omega,T) = \chi''(q=0,\omega,T,t=0) \tag{S2}$$

$$= b^{\gamma/\nu}\chi''(q=0, b^z\omega, b^zT), \tag{S3}$$

since $b$ is arbitrary, we can choose $b^zT = 1$, $b = T^{-1/z}$. It then follows that

$$\chi''(q=0,\omega,T) = T^{-\frac{\gamma}{\nu z}}\phi_1\left(\frac{\omega}{T}\right), \tag{S4}$$

$\phi_1(x)$ is a scaling function and we can collapse data onto a single trend with a suitable choice of $\frac{\gamma}{\nu z}$.

From Eqn. S1, we have for $t = 0$,

$$\chi(q,\omega,T) = b^{\gamma/\nu}\chi(bq, b^z\omega, b^zT). \tag{S5}$$

Assuming a linear susceptibility near $\omega = 0$, the low-frequency slope is:

$$\left.\frac{\chi''(q,\omega,T)}{\omega}\right|_{\omega\to 0} = b^{\gamma/\nu}b^z \left.\frac{\chi''(bq, b^z\omega, b^zT)}{b^z\omega}\right|_{b^z\omega\to 0}. \tag{S6}$$

Again using $b^zT = 1$,

$$\left.\frac{\chi''(q,\omega,T)}{\omega}\right|_{\omega\to 0} = T^{-\left(\frac{\gamma}{\nu z}+1\right)} \left.\frac{\chi''(T^{-\frac{1}{z}}q,\omega,1)}{\omega}\right|_{\omega\to 0}, \tag{S7}$$

$$= T^{-\left(\frac{\gamma}{\nu z}+1\right)}\phi_2(T^{-\frac{1}{z}}q) \tag{S8}$$

where

$$\phi_2(x) = \left.\frac{\chi''(x,\omega,1)}{\omega}\right|_{\omega\to 0}. \tag{S9}$$

(S10)

If $\phi_2(x)$ is a function peaked at the ordering wavevector $q = 0$ with width $w$. We can determine $z$ from the temperature dependence of the width

$$w = \xi^{-1} \propto T^{\frac{1}{z}}. \tag{S11}$$

### Phenomenological susceptibility for spin fluctuations

We parameterize our normal-state data with a phenomenological susceptibility used by Aeppli *et al.* [1] :

$$\chi''(\mathbf{Q},\omega) = \chi''(\mathbf{Q}_\delta,\omega)\frac{\kappa^4(\omega)}{[\kappa^2(\omega)+R(\mathbf{Q})]^2}, \tag{S12}$$

where

$$R(\mathbf{Q}) = \frac{1}{4\delta^2}\big\{[(H-\tfrac{1}{2})^2+(K-\tfrac{1}{2})^2-\delta^2]^2 + 4(H-\tfrac{1}{2})^2(K-\tfrac{1}{2})^2\big\}. \tag{S13}$$

$R(\mathbf{Q})$ has zeros at the positions $\mathbf{Q}_\delta = (1/2\pm\delta, 1/2)$ and $(1/2\pm\delta, 1/2)$ and this function approximately reproduces the $\mathbf{Q}$ dependence of our data. Near each $\mathbf{Q}_\delta$, $R(\mathbf{Q}_\delta+\mathbf{q}) = |\mathbf{q}|^2$. Therefore,

$$\lim_{|\mathbf{q}|\to 0}\chi''(\mathbf{Q},\omega) = \frac{\chi''(\mathbf{Q}_\delta,\omega)}{[1+\kappa^{-2}(\omega)\,|\mathbf{q}|^2]^2} \tag{S14}$$

and we can we can interpret $\kappa^{-1}(\omega)$ as a "dynamic correlation length" with usual static correlation length given by $\xi = \kappa^{-1}(\omega)$.

$\kappa(\omega, T)$ *model*

$$\kappa^2(\omega) = \Delta + a_0^{-2}\left[\left(\frac{\hbar\omega}{E_\kappa}\right)^{2/z} + r\left(\frac{k_B T}{E_\kappa}\right)^{2/z}\right] \tag{S15}$$

We fit $\kappa(\omega, T)$ in units of $\text{Å}^{-1}$ to the model in Eqn. S15 fixing $r$ to be 1 as has been found to be approximately true in LSCO x=0.14 [1]. Here $\Delta$ is a tuning parameter which is zero for a QCP, $E_\kappa$ is an energy scale and $a_0$ is the in-plane lattice parameter. This fit gives $z = 1.83 \pm 0.35$, $\Delta = (4 \pm 14) \times 10^{-4}\text{Å}^{-2}$ and $E_\kappa = 68 \pm 17$ meV. Thus $\Delta$ is zero within the resolution of the experiment.

### Quantum phase transitions in metals with Harris disorder

This section recalls the theoretical model presented in Ref. [2], and describes the computation of its real frequency response functions. There is some overlap of the initial discussion here with the review in Ref. [3].

We focus on quantum fluctuations of the spin density wave (SDW) order parameter across the quantum phase transition from the Fermi liquid [4, 5]. We write the SDW order as $(a = x, y, z)$

$$S_a(\mathbf{r}) = \sum_\ell \phi_{\ell a} e^{i\mathbf{Q}_{\delta\ell}\cdot\mathbf{r}} \tag{S16}$$

where $S_a$ is the electron spin at position $\mathbf{r}$, $\ell = 1\ldots 4$ labels the 4 ordering wavevectors (fix this) $\mathbf{Q}_{\delta\ell}$ at $(1/2, 1/2 \pm \delta)$ and $(1/2 \pm \delta, 1/2)$. We are interested in fluctuations of the SDW order parameters $\phi_{\ell a}$ coupled to electrons $c_{\mathbf{k}\sigma}$ with dispersion $\varepsilon(\mathbf{k})$ which has a Fermi surface. Including the effects of spatial disorder, we have a two-dimensional Yukawa-Sachdev-Ye-Kitev model with the imaginary time $(\tau)$ Lagrangian [6, 7]

$$\begin{aligned}\mathcal{L}_{YSYK} = &\sum_{\mathbf{k}} c^\dagger_{\mathbf{k}\sigma}\left(\frac{\partial}{\partial\tau} + \varepsilon(\mathbf{k})\right) c_{\mathbf{k}\sigma} + \int d^2\mathbf{r}\,\Big\{\lambda\,[\phi(\mathbf{r})]^2 \\ &+ [g + g'(\mathbf{r})]\sum_\ell c^\dagger_\sigma(\mathbf{r})\tau^a_{\sigma\sigma'}c_{\sigma'}(\mathbf{r})\,\phi_{\ell a}(\mathbf{r})e^{i\mathbf{Q}_{\delta\ell}\cdot\mathbf{r}} \\ &+ K\,[\nabla_{\mathbf{r}}\phi(\mathbf{r})]^2 + u\,[\phi(\mathbf{r})]^4 + v(\mathbf{r})c^\dagger_\sigma(\mathbf{r})c_\sigma(\mathbf{r})\Big\}\,.\end{aligned} \tag{S17}$$

Here $\tau^a$ are the Pauli matrices, $\lambda$ is the parameter employed to tune across the transition, and $g$ is the Yukawa coupling between the fermions and bosons. We have included two sources of spatial randomness. The spatially random potential $v(\mathbf{r})$, with ensemble averages $\overline{v(\mathbf{r})} = 0$, $\overline{v(\mathbf{r})v(\boldsymbol{r}')} = v^2\delta(\mathbf{r} - \boldsymbol{r}')$, acts on the fermion density, and plays a central role in the theory of disorder-induced electron localization [8]. Such fermion localization effects are also present here, but all indications are that such effects are not important for the cuprates. Instead, our focus will be on the more relevant 'Harris disorder', induced by spatial randomness in the position of the quantum critical point. Following Ref. [7], we have represented this by a spatially random Yukawa coupling $g'(\mathbf{r})$ with $\overline{g'(\mathbf{r})} = 0$, $\overline{g'(\mathbf{r})g'(\boldsymbol{r}')} = g'^2\delta(\mathbf{r} - \boldsymbol{r}')$. Such Harris disorder can lead to boson localization at low temperatures [2, 9], where it must be treated non-perturbatively, as we do below. But in higher temperature regimes, where the bosons do not localize, we can add a large number of flavor labels to the fields so that (S17) is amenable to a large flavor solution [6, 7, 10].

Patel *et al.* [9] have studied the YSYK model (S17) at $g = 0$ by large scale, high precision quantum Monte Carlo simulations (with no additional flavors), and their results for the imaginary time spin susceptibility appear in Fig. 4E of the main text. We describe below use the approach of Ref. [2] which treats the interactions in a mean-field manner, but accounts for disorder numerically exactly; this approach has the advantage of allowing exact analytic continuation to real frequencies at arbitrary temperatures. The results of Ref. [2] are in general agreement with the exact Monte Carlo results of Ref. [9]: both show an extended quantum Griffiths phase with $\omega/T$ scaling, but the value of $\alpha$ is smaller and more reliable in the Monte Carlo study.

The approach of Ref. [2] is to integrate out the fermions from (S17) (assuming fermionic eigenmodes remain extended), and consider the resulting Landau-damped Hertz-Millis theory for the boson $\phi$ alone. The spatial disorder in the Yukawa coupling $g'(\mathbf{r})$ will lead to disorder in all couplings in the effective boson theory. For simplicity, we retain only the most relevant 'random mass' disorder in the tuning parameter $\lambda \to \lambda + \delta\lambda(\mathbf{r})$. We also drop the longer-range RKKY couplings between the $\phi$ that will be induced by integrating out the fermions [11]. We discretize the boson theory on a lattice of sites (labeled by $j$), and write the SDW order parameters in terms of a real $\phi$ with a single index $a = 1\ldots M$ with $M = 12$. In this manner, we obtain the action

$$\begin{aligned}\mathcal{S} =&\mathcal{S}_\phi + \mathcal{S}_{\phi d} \\ \mathcal{S}_\phi =&\int d\tau\left[\frac{J}{2}\sum_{\langle ij\rangle}(\phi_{ia} - \phi_{ja})^2 + \right. \\ &\left.\sum_j\left\{\frac{\lambda + \delta\lambda_j}{2}\phi^2_{ja} + \frac{u}{4M}\left(\phi^2_{ja}\right)^2\right\}\right] \\ \mathcal{S}_{\phi d} =&\frac{T}{2}\sum_\Omega\sum_j\left(\gamma|\Omega| + \Omega^2/c^2\right)|\phi_{ja}(i\Omega)|^2\,,\end{aligned} \tag{S18}$$

where $\Omega$ is a Matsubara frequency at a temperature $T$, $\gamma$ is the Landau damping, and the $\Omega^2/c^2$ term has been inserted as a high frequency cutoff. The random mass disorder satisfies $\overline{\delta\lambda(\mathbf{r})} = 0$, $\overline{\delta\lambda(\mathbf{r})\delta\lambda(\boldsymbol{r}')} = \delta\lambda^2\delta(\mathbf{r} - \boldsymbol{r}')$. For simplicity, we have assumed a global $\mathrm{O}(M)$ symmetry, but this assumption can be relaxed without significantly modifying the results.

The theory in (S18) has been studied using a strong disorder renormalization group [12–14]. But the same basic results are obtained by the method of Ref. [2] (originally used for a related problem in $d = 1$ in Ref. [15]), which also allows study of the crossover at higher energies to weak disorder, and this will be important for our purposes. Following Refs. [2, 15], we replace $\mathcal{S}_\phi$ by an effective quadratic action, while renormalizing the space dependent mass in a self-consistent manner; this leads to

$$\begin{aligned}\widetilde{\mathcal{S}}_\phi &= \int d\tau \Big[\frac{J}{2}\sum_{\langle ij\rangle}(\phi_{ia}-\phi_{ja})^2 + \sum_j \frac{\widetilde{\lambda}_j}{2}\phi_{ja}^2\Big] \\ \widetilde{\lambda}_j &= \lambda + \delta\lambda_j + \frac{u}{M}\sum_a \left\langle \phi_{ja}^2 \right\rangle_{\widetilde{\mathcal{S}}_\phi + \mathcal{S}_{\phi d}} \\ &= \lambda + \delta\lambda_j + uT\sum_\Omega \sum_b \frac{\psi_{bi}\psi_{bj}}{\gamma|\Omega| + \Omega^2/c^2 + e_b}\,,\end{aligned} \tag{S19}$$

where $e_b$ and $\psi_{bj}$ are eigenvalues and eigenfunctions of the $\phi$ quadratic form in $\widetilde{\mathcal{S}}_\phi$, labeled by the index $b = 1 \ldots L^2$ for a $L \times L$ sample. For each disorder realization $\delta s_j$, the values of $\widetilde{\lambda}_j$ are determined by numerically solving (S19), and this also yields results for the eigenvalues $e_b$ and the eigenvectors $\psi_{bj}$. The dynamic spin susceptibility is then computed at a real frequency $\omega$ from

$$\chi_{ij}(\omega) = \sum_b \frac{\psi_{bi}\psi_{bj}}{-i\gamma\omega - \omega^2/c^2 + e_b}\,, \tag{S20}$$

followed by a Fourier transform from spatial co-ordinates to momenta.

Results from the computation above are presented in Fig. 4 of the main text, and Figs. S1-S9 below. The chosen parameter values are $J = 1$, $\gamma = 1$, $c^2 = 10$, $u = 1$ and $\delta\lambda^2 = 0.25$. The quantum critical point at $T = 0$ is at $\lambda_c = -0.4586$ [2]. We used a system size of $160 \times 160$ and averaged over 20 disorder realizations. We can set the energy scale by identifying the highest energy energy spin excitation ($c\sqrt{8J} \approx 9$ with the highest energy spin wave ($\approx 300$ meV [16]). This leads to the estimate $300/9 \approx 33$ meV as the unit of energy for the numerics.

The results for the dynamic spin susceptibility at the ordering wavevector $\mathbf{Q}_\delta$ were shown in Fig. 4 of the main text for $\lambda = \lambda_c$, where we found good $\omega/T$ scaling. Fig. S1 extends these results to $\lambda > \lambda_c$. Now we find $\omega/T$ scaling only for smaller values of $\omega/T$. This restriction of $\omega/T$ scaling to $\omega \lesssim T$ for $\lambda > \lambda_c$ is not at odds with the experimental results in the main text, which also, strictly speaking, establish $\omega/T$ scaling for $\omega \lesssim T$ as the range of $\omega$ values available is not enough to achieve larger values of $\omega/T$ at the larger values of $T$ that are considered.

The value of the exponent $\alpha$ decreases monotonically with increasing distance from the critical point (increasing $\lambda$). In Fig. S2, we show that using a smaller value of $\alpha$ makes little difference to the quality of the fit at small $\omega/T$, which is the region at which scaling is established in the observations.

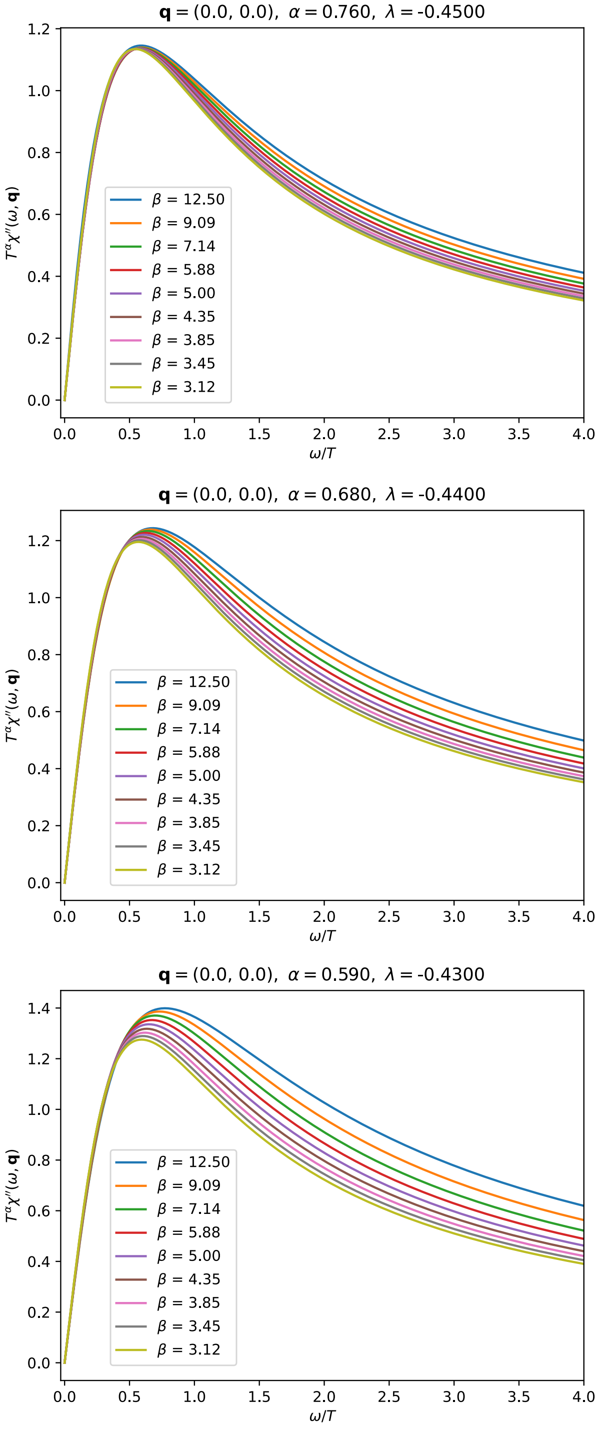


Fig. S1: **Scaling plots of the dynamic spin susceptibility at the ordering wavevector for** $\lambda > \lambda_c = -0.4586$. Results for $\lambda = \lambda_c$ are in Fig. 4B in the main text.

Fig. S3 shows similar results for the *local* dynamic spin

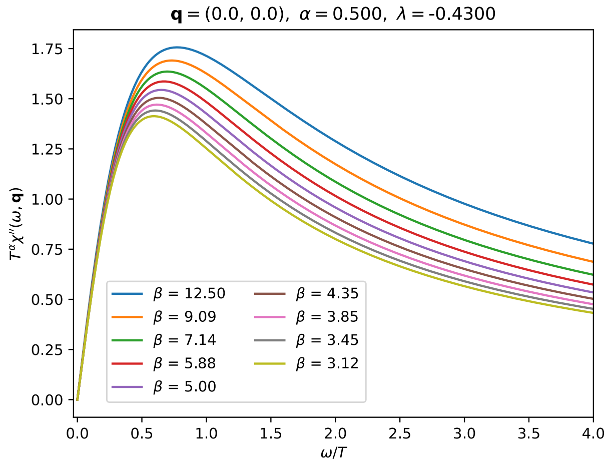


Fig. S2: **Scaling plots of the dynamic spin susceptibility at the ordering wavevector for** $\lambda = -0.43$. A smaller value of the exponent $\alpha$ is used in comparison to the corresponding plot in Fig. S1.

susceptibility

$$\chi''_L(\omega) = \int \frac{d^2\mathbf{q}}{4\pi^2}\chi''(\boldsymbol{q},\omega) \tag{S21}$$

for $\lambda \geq \lambda_c$. Now we find that $\omega/T$ scaling holds for all values $\lambda$, an indication that the criticality for $\lambda > \lambda_c$ is from localized spin fluctuations. This is just as expected from a quantum Griffiths critical phase. By scaling, the exponent for the local susceptibility $\alpha + \mu = 2/z$, and this is consistent with our values $\mu = 0.1$ to $0.16$, $\alpha = 0.84$ to $0.59$ and $z = 2.1$ to $2.6$ respectively for the range of $\lambda = -0.4586$ to $-0.4300$ considered.

Fig. S4 extends the analysis of scaling for the local and ordering wavevector susceptibilities at $\lambda = \lambda_c$ to much lower values of $T$, showing a breakdown of $\omega/T$ scaling at low $T$. This is consistent with results for the boson density of states in Ref. [9], which showed a crossover from the constant density of states associated with marginal Fermi liquid behavior at higher energy, to a regime dominated by Griffiths effects at lower energy. The breakdown of $\omega/T$ scaling here in the dynamic spin susceptibility likely arises from the enhanced boson density of states at smallest energies, and could possibly be captured by experiments at lower temperatures than the ones considered in this work.

Next, we turn to the behavior of the inverse correlation length, $\kappa$, defined by (6) in the main text (also (S12)), which we adapted to

$$\frac{\chi''(\mathbf{q},\omega)}{\chi''(\mathbf{q}=0,\omega)} = \frac{\kappa^4(\omega)}{[\kappa^2(\omega) + 4 - 2\cos(q_x) - 2\cos(q_y)]^2}\,. \tag{S22}$$

Fig. S5 shows that (S22) provides an excellent fit to the numerical data, and this enables determination of

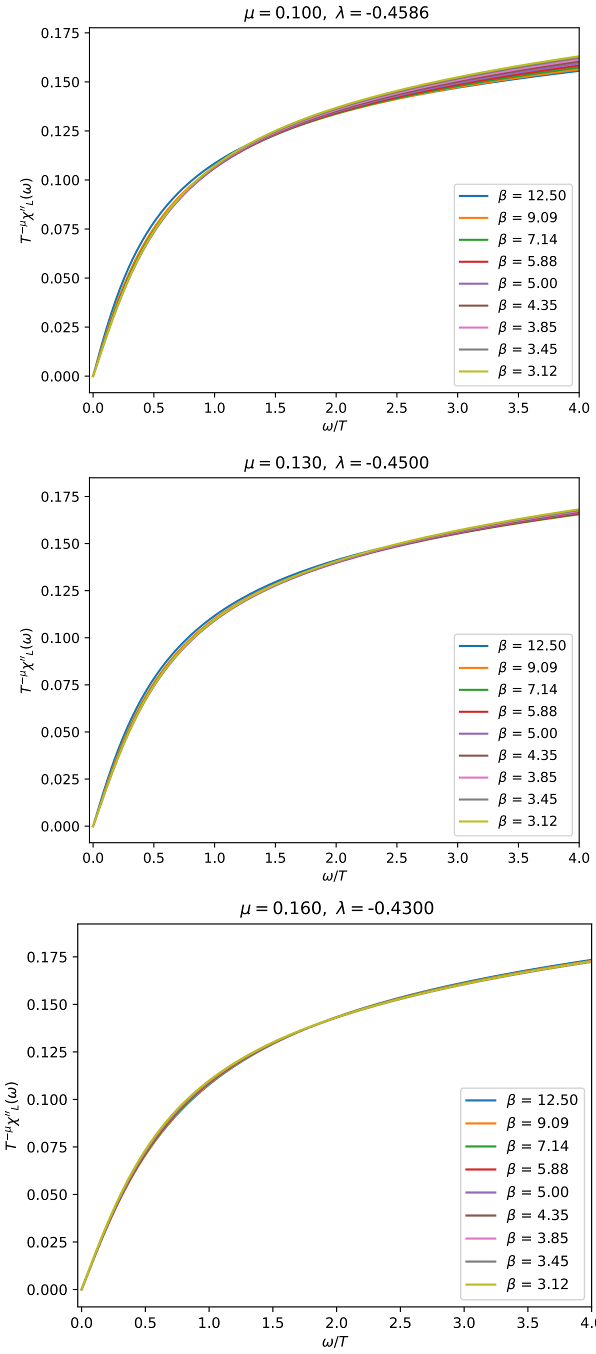


Fig. S3: **Scaling plots of the local dynamic spin susceptibility for** $\lambda \geq \lambda_c = -0.4586$.

$\kappa(\omega, T)$. Our results for $\kappa$ and their scaling are shown in Fig. 4C,D of the main text at $\lambda = \lambda_c$. Corresponding results for $\lambda > \lambda_c$ appear in Figs. S6 and S7. As for the dynamics spin susceptibility at the ordering wavevector, $\omega/T$ scaling works for $\lambda = \lambda_c$, but only for smaller values of $\omega/T$ for $\lambda > \lambda_c$. The plots of Fig. S7 are shown on a logarithmic frequency scale in Fig. S8 (as in Figs. 3 and 4D of the main text), which exposes the lower frequency

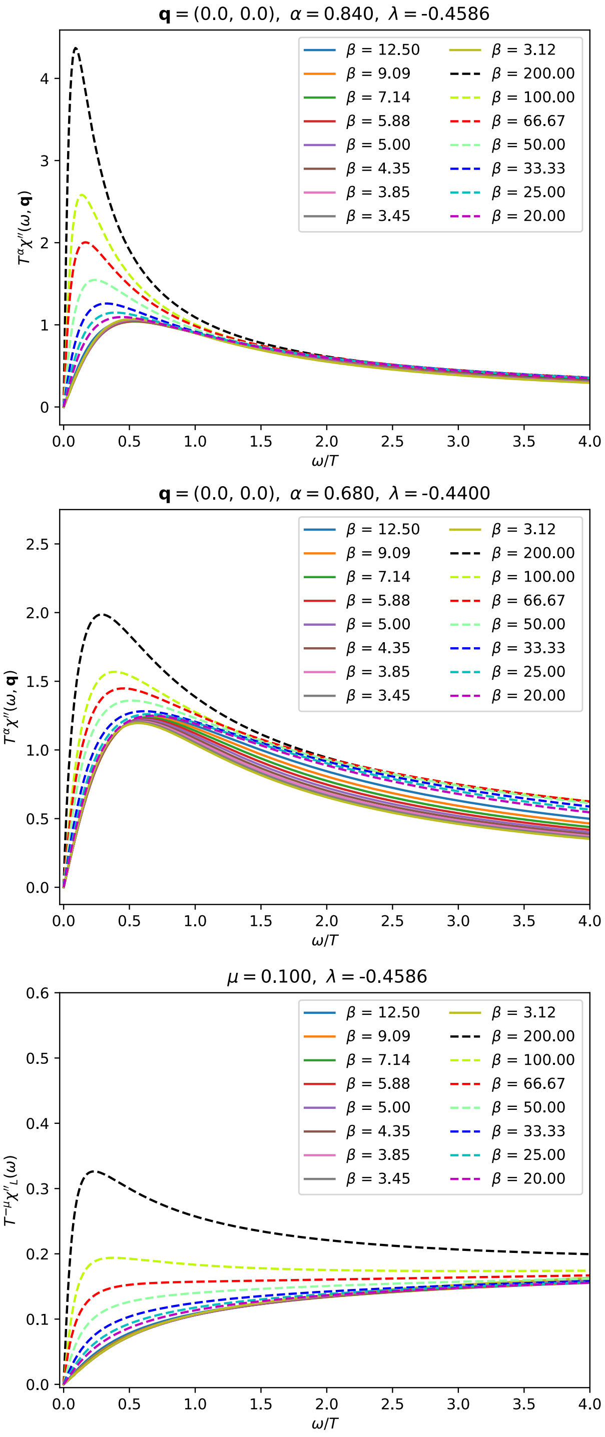


Fig. S4: **Breakdown of scaling at very low temperatures**. The dynamic susceptibilities at lower temperatures. Compare to the plots in Fig. 4 of the main text and Fig. S3.

range.

Finally, we complement plots of the resistivity induced by the disordered spin fluctuations in Fig. 4 of the main text at additional values of $\lambda$ in Fig. S9. The resistivity

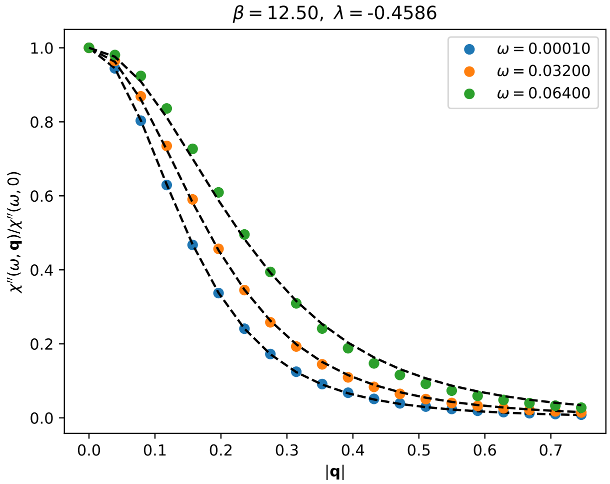


Fig. S5: **Fits of the dynamic spin susceptibility to (6) in the main text, allowing determination of $\kappa(\omega, T)$.**

was computed from the numerical results for $\chi''_L(\omega)$, as specified in Ref. [2].

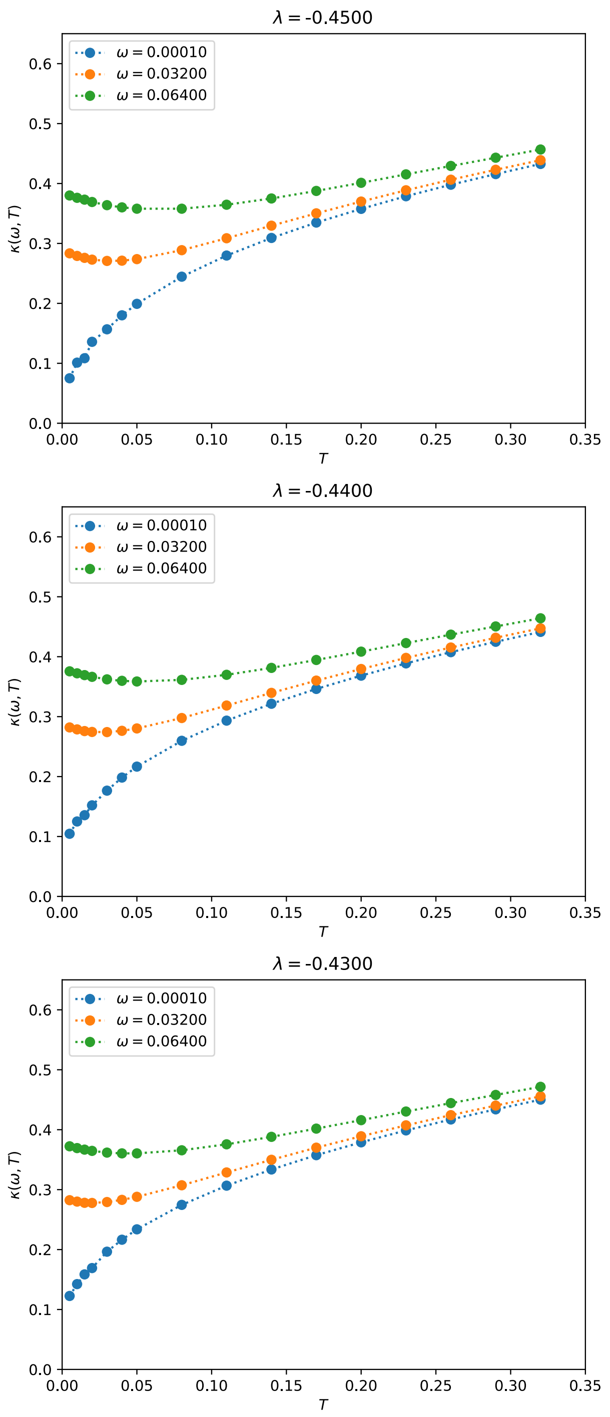


Fig. S6: **Plots of $\kappa$ for $\lambda > \lambda_c = -0.4586$.** Results for $\lambda = \lambda_c$ are in Fig. 4C in the main text.

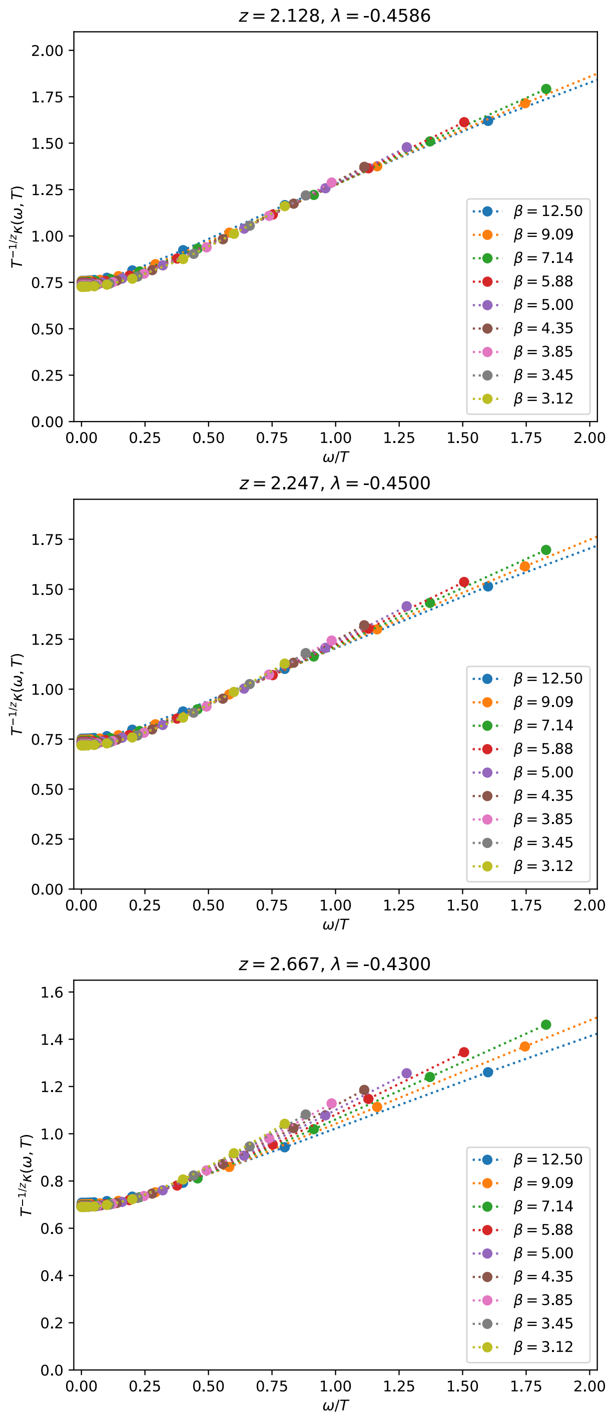


Fig. S7: **Scaling plots of $\kappa$ for $\lambda \geq \lambda_c = -0.4586$.**

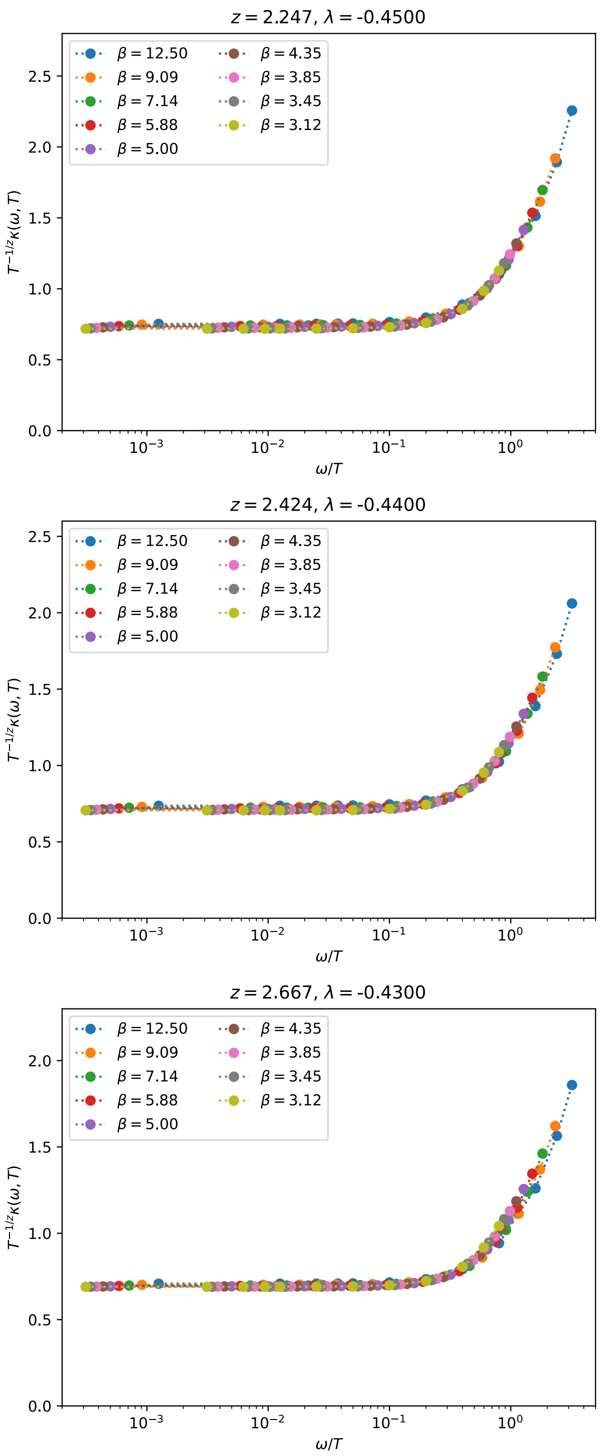


Fig. S8: **Scaling plots of $\kappa$ for $\lambda > \lambda_c = -0.4586$.** As in Fig. S7, but with a logarithmic frequency axis. Compare to the experimental results in Figs. 3E and 4D of the main text.

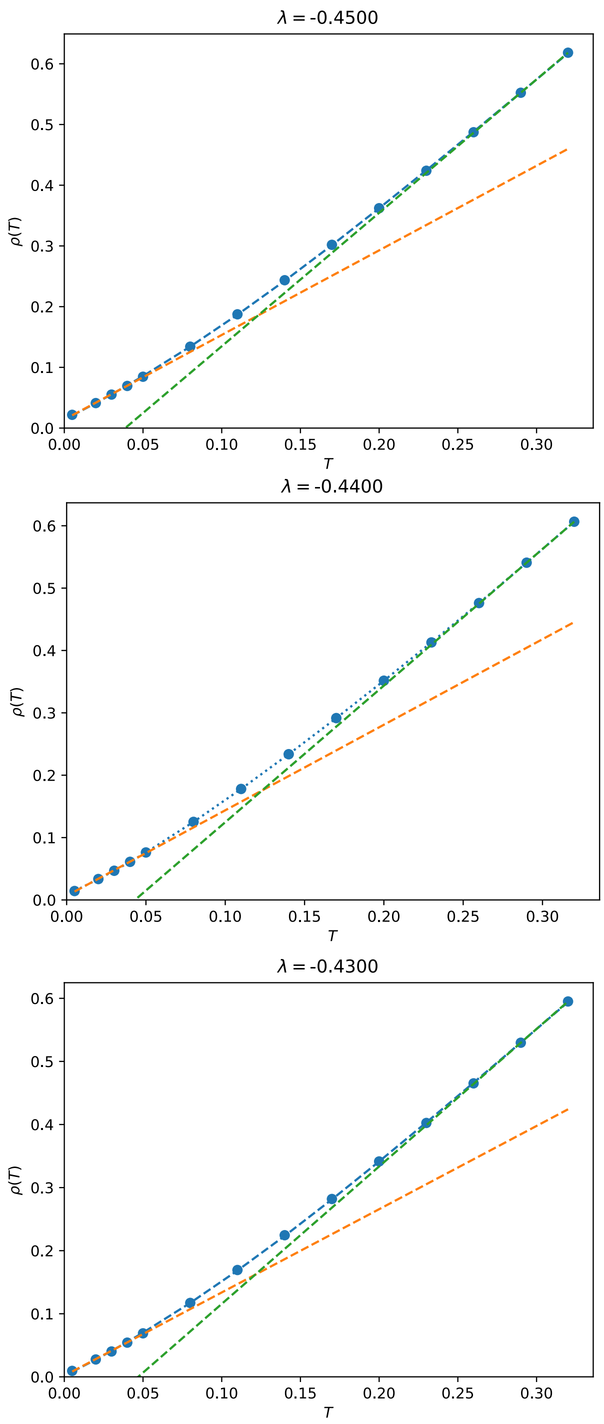


Fig. S9: **Resistivity as a function of temperature**. As in Fig. 4F of the main text.

## EXPERIMENTAL METHODS

### Single-crystal sample growth and characterization

Single crystals of $La_{2-x}Sr_xCuO_x$ (x = 0.22) were grown by the travelling-solvent floating-zone method. The crystals were annealed in 1 bar of flowing oxygen at 800°C for six weeks. The Sr concentration was determined by scanning electron microscopy with electron probe microanalyzer (SEM-EPMA) and inductively coupled plasma atomic emission spectroscopy (ICP-AES) to be x = 0.215 ± 0.005. SQUID magnetometry measurements show that $T_{c,\mathrm{onset}}$=26K. The sample consists of 29.8g of LSCO crystal, mounted and co-aligned using the ALF single crystal diffractometer.

### Inelastic neutron scattering

Inelastic neutron scattering measurements were performed at the LET direct time-of-flight spectrometer at ISIS. LET is a multiplexing instrument which allows for simultaneous collection of data at multiple neutron incident energies. Three fixed incident energies $E_i = 3.76$, 6.82, 16.02 meV were used for the whole data collection.

To this end, the sample was mounted with its $c$-axis vertical and the azimuthal angle swept over a range of ∼108° about the region of interest. Measurements were taken at one degree intervals to ensure adequate coverage over the entire region around the (1/2,1/2) wavevector.

Two experiments were performed. In 'Experiment 1' we measure at 5 different temperatures including room temperature (290K) and the superconducting transition temperature (26K). In Experiment we measured at 3 of the 5 original temperatures with the sample rotated by 90° with respect to Experiment 1 and counted for a longer period at 300 K.

### Data Analysis

The scattering cross-section is related to the scattering function $S(\mathbf{Q},\omega)$ and energy- and wavevector-dependent magnetic response function $\chi''(\mathbf{Q},\omega)$ by the fluctuation-dissipation theorem

$$\frac{k_i}{k_f}\frac{d^2\sigma}{d\Omega\, dE} = S(\mathbf{Q},\omega) = \frac{2(\gamma r_e)^2}{\pi g^2 \mu_B^2}|F(\mathbf{Q})|^2 \frac{\chi''(\mathbf{Q},\omega)}{1-\exp(-\hbar\omega/k_BT)}, \tag{S23}$$

where $(\gamma r_e)^2 = 0.2905$ barn sr$^{-1}$, and $F(\mathbf{Q})$ the magnetic form factor.

Counts measured at position sensitive detectors were normalized to a vanadium standard to correct for differences in detector efficiency and then used to reconstruct the momentum and energy-dependent scattering function $S(\mathbf{Q},\omega)$. This process was repeated for each $E_\mathrm{i}$ producing three 4-D datasets at each temperature.

#### *2-D Q Slices*

Our data analysis procedure involved generating 11 slices across the three $E_\mathrm{i}$s over the energy range $\Delta E \sim 1-10$ meV. Data is binned over $L = \pm 1$ and $E = \hbar\omega \pm 0.5$ meV. The scattering function is converted to $\chi''(\mathbf{Q},\omega)$ using Eqn. S23 following subtraction of a q-independent background. This background is determined through least-squares fitting (see section Cuts).

#### *1-D Q Cuts*

In order to parameterise the excitations for a given $\omega, T$, we use a further rebinning of the data slices. Two cuts through the high $|\mathbf{Q}|$ and low $|\mathbf{Q}|$ peaks, respectively at $\{(1/2,1/2-\delta), (1/2-\delta,1/2)\}$ and $\{(1/2,1/2+\delta), (1/2+\delta,1/2)\}$, are generated from each slice by binning along the $\mathbf{Q}$-direction perpendicular to the cut (see Fig. 1D in the main text).

Finally, we carry out a resolution-corrected least-squares fit (see Fig. S10) to each cut using the Tobyfit module in Horace [17]. The susceptibility is modelled by Eqn. S12. This has two energy-dependent parameters $\chi''(\mathbf{Q}_\delta,\omega)$ and $\kappa(\omega)$ which control the height and width of the peaks in $\mathbf{Q}$ respectively. The incommensurability $\delta$ of the excitations also enters into the model via $R(\mathbf{Q})$.

The value of $\delta$ in Eqn. S13 was fixed for each temperature. The fitted values ranged from $\delta = 0.139$ to $\delta = 0.131$ for $T = 26$ and 300 K respectively. When making $T$-dependent (scaling) plots we evaluated the fitted $\chi''(\mathbf{Q}_\delta,\omega)$ for the $T = 26$ K value of $\delta$. in the final fits but found to have a slight systematic decrease from $\delta = 0.139$ to $\delta = 0.131$ over the range 26K to 300K. This was determined by averaging over energy dependent best-fit values below 5meV where the peaks are sharp. We also fit a q-independent background in the model structure factor for each cut.

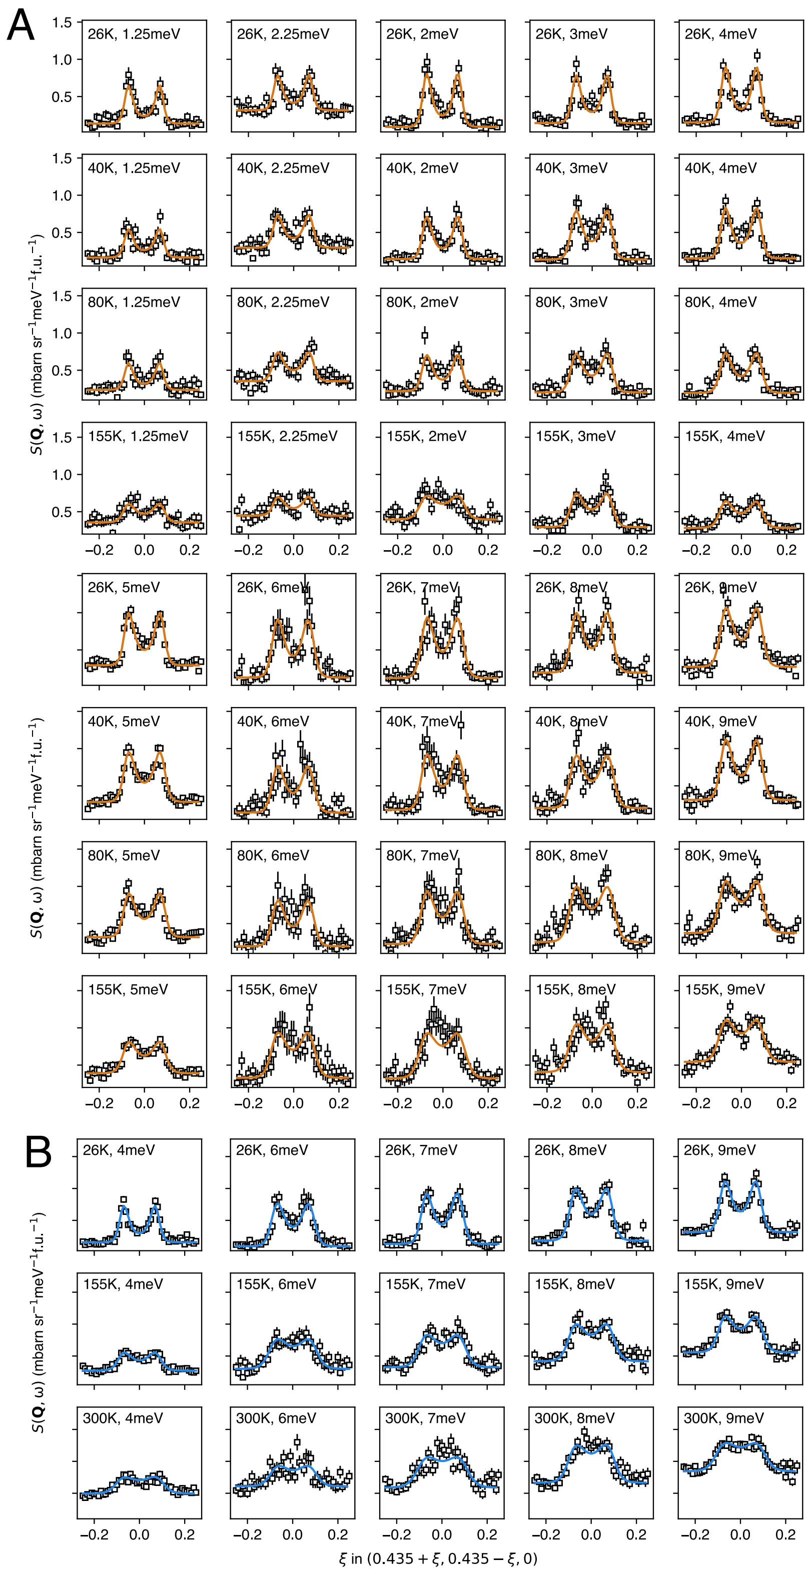


Fig. S10: A representative selection of $S(\mathbf{Q},\omega)$ cuts and fits to the model described in the main text. (**A**) Experiment 1. (**B**) Experiment 2.

[1] G. Aeppli, T. Mason, S. Hayden, H. Mook, and J. Kulda, Science **278**, 1432 (1997).

[2] A. A. Patel, P. Lunts, and S. Sachdev, Proceedings of the

National Academy of Sciences **121**, e2402052121 (2024).
[3] S. Sachdev, "The foot, the fan, and the cuprate phase diagram: Fermi-volume-changing quantum phase transitions," (2025), arXiv:2501.16417 [cond-mat.str-el].
[4] J. A. Hertz, Phys. Rev. B **14**, 1165 (1976).
[5] A. J. Millis, Phys. Rev. B **48**, 7183 (1993).
[6] I. Esterlis, H. Guo, A. A. Patel, and S. Sachdev, Phys. Rev. B **103**, 235129 (2021).
[7] A. A. Patel, H. Guo, I. Esterlis, and S. Sachdev, Science **381**, 790 (2023).
[8] P. A. Lee and T. V. Ramakrishnan, Rev. Mod. Phys. **57**, 287 (1985).
[9] A. A. Patel, P. Lunts, and M. S. Albergo, "Strange metals and planckian transport in a gapless phase from spatially random interactions," (2024), arXiv:2410.05365 [cond-mat.str-el].
[10] C. Li, D. Valentinis, A. A. Patel, H. Guo, J. Schmalian, S. Sachdev, and I. Esterlis, Phys. Rev. Lett. **133**, 186502 (2024).
[11] J. H. Van Vleck, Rev. Mod. Phys. **34**, 681 (1962).
[12] J. A. Hoyos, C. Kotabage, and T. Vojta, Phys. Rev. Lett. **99**, 230601 (2007).
[13] T. Vojta, C. Kotabage, and J. A. Hoyos, Phys. Rev. B **79**, 024401 (2009).
[14] T. Vojta, in *Lectures on the Physics of Strongly Correlated Systems XVII: Seventeenth Training Course in the Physics of Strongly Correlated Systems*, American Institute of Physics Conference Series, Vol. 1550, edited by A. Avella and F. Mancini (AIP, 2013) pp. 188–247, arXiv:1301.7746 [cond-mat.dis-nn].
[15] A. Del Maestro, B. Rosenow, M. Müller, and S. Sachdev, Phys. Rev. Lett. **101**, 035701 (2008).
[16] S. M. Hayden, G. Aeppli, R. Osborn, A. D. Taylor, T. G. Perring, S. W. Cheong, and Z. Fisk, Phys. Rev. Lett. **67**, 3622 (1991).
[17] R. Ewings, A. Buts, M. Le, J. van Duijn, I. Bustinduy, and T. Perring, Nuclear Instruments and Methods in Physics Research Section A: Accelerators, Spectrometers, Detectors and Associated Equipment **834**, 132 (2016).
